# Supplementary material for: Stabilization of competing ferroelectric phases of HfO$_2$ under epitaxial strain
Source: arXiv:2001.08692 ancillary file (2020-09-26)
Supplement: Supplementary file 1 [file Supplementary_Materials.pdf]

# Supplementary Materials

Yubo Qi[1], Sobhit Singh[1], Claudia Lau[2], Fei–Ting Huang[1], Xianghan Xu[1]
Frederick J. Walker[2], Charles H. Ahn[2], Sang–Wook Cheong[1], and Karin M. Rabe[1]
[1]Department of Physics & Astronomy, Rutgers University, Piscataway, New Jersey 08854, USA
[2]Department of Physics, Yale University, New Haven, Connecticut 06520, USA

## I. NUMERICAL DETAILS

Density-Functional Theory (DFT) based first-principles calculations are carried out using the QUANTUM–ESPRESSO [S1] plane–wave DFT code within the generalized gradient approximation (GGA). The plane–wave cutoff energy is 50 Ry, and the the Brillouin zone is sampled by a 4×4×4 Monkhorst–Pack $k$–point mesh [S2]. Atomic forces were converged when a maximum threshold of $5\times10^{-3}$ eV/Å per atom is reached. All the reported structures, energies and polarization values were obtained using the QUANTUM–ESPRESSO code.

In order to test the dynamical and elastic stability of the studied structures, we have performed complementary DFT calculations of phonon dispersion relations and elastic constants using Projector Augmented Wave (PAW) method [S3] as implemented in the VASP software [S4–S6]. We considered four valence electrons of Hf ($6s^2 6d^2$) and six valence electrons of O ($2s^2 2p^4$) in the PAW pseudo-potential. The exchange-correlation energy was computed within the LDA. An energy cutoff of 600 eV was used for the plane wave basis set and a $8\times8\times8$ $k$-mesh was used to sample the reciprocal space. $10^{-8}$ eV was used for the energy convergence criterion for all self-consistent DFT calculations and $10^{-4}$ eV/Å was used as the force convergence criterion for structural relaxations performed within the VASP code. Phonon calculations were performed using the finite-displacement approach and the PHONOPY software [S7] was used to evaluate the force constants. A supercell of size $2\times2\times2$ was used for phonon calculations. The elastic stability of the studied structures was tested using the MECHELASTIC code [S8].

## II. THE PSEUDOCUBIC LATTICE CONSTANTS GIVEN BY GGA AND EXP.

| phase | $a$ | $b$ | $c$ |
|---|---|---|---|
| c (GGA) | 5.04 | 5.04 | 5.04 |
| c (EXP)[a] | 5.08 | 5.08 | 5.08 |
| t (GGA) | 5.04 | 5.04 | 5.20 |
| t (EXP)[b] | 5.06 | 5.06 | 5.20 |
| oIII (GGA) | 5.05 | 5.01 | 5.24 |
| oIII (EXP) | N/A | N/A | N/A |
| m (GGA) | 5.29 | 5.10 | 5.15 |
| m (EXP)[b] | 5.29 | 5.12 | 5.17 |
| oIV (GGA) | 5.08 | 5.08 | 5.16 |
| oIV (EXP) | N/A | N/A | N/A |

[a] Reference [S9]; [b] Reference [S10];

TABLE S1. Comparison between the lattice constants given by GGA and experiments. The maximum error is less than 0.8%.

## III. PHONON DISPERSION OF THE oIII AND oIV PHASES

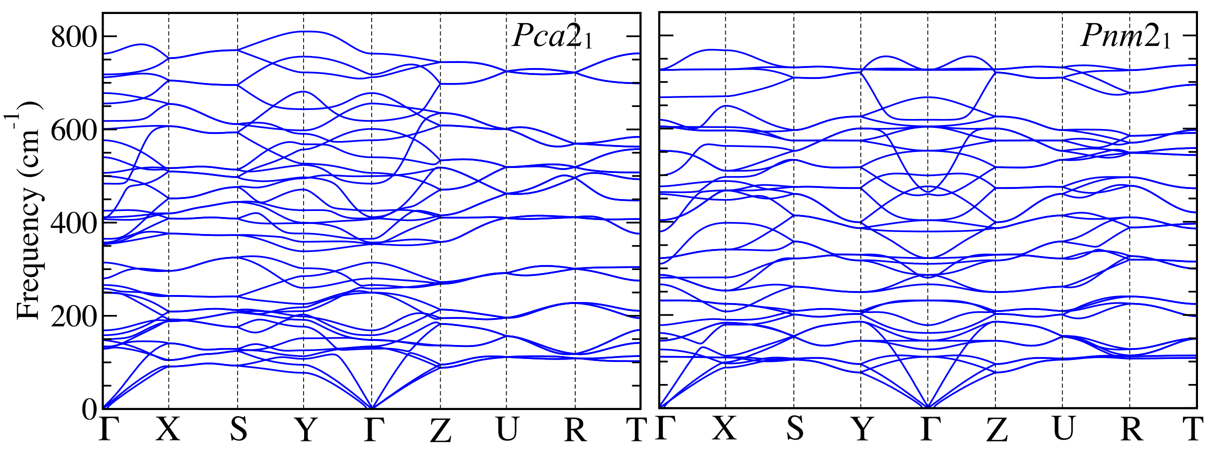


FIG. S1. The DFT (LDA) calculated phonon dispersion for the $Pca2_1$ (oIII) and (111)–oriented $Pnm2_1$ (oIV) structures. The atomiic positions of the optimized structures for the oIII– and oIV phases are listed in TABLE S4 and S5. Calculated phonon dispersion confirms the dynamical stability of the studied structures.

## IV. ELASTIC AND MECHANICAL PROPERTIES

| Phase | $C_{11}$, $C_{12}$, $C_{13}$, $C_{22}$, $C_{23}$, $C_{33}$, $C_{44}$, $C_{55}$, $C_{66}$ | Mechanical stability test |
|---|---|---|
| oIII-phase | 470.6, 197.0, 154.7, 442.3, 154.5, 419.3, 101.9, 110.2, 153.3 | Pass |
| oIV-phase | 457.3, 190.7, 183.2, 525.9, 180.3, 531.0, 64.6, 120.8, 123.8 | Pass |

TABLE S2. This table contains the DFT–LDA calculated elastic constants ($C_{ij}$, in GPa units) of the oIII and oIV phases together with the result of Born-Huang mechanical stability test performed using the MechElastic code [S8]. The elastic constants were converged better than 1 GPa by increasing the size of $k$-mesh.

| Elastic Modulus | oIII-phase | oIV-phase |
|---|---|---|
| Bulk modulus (GPa) | 259.6 | 290.6 |
| Shear modulus (GPa) | 126.5 | 116.2 |
| Young modulus (GPa) | 326.5 | 307.4 |
| P-wave modulus (GPa) | 428.3 | 445.5 |
| Poisson ratio | 0.29 | 0.32 |
| Bulk/Shear ratio | 2.1 (ductile) | 2.5 (ductile) |

TABLE S3. This table contains the DFT–LDA calculated values of various elastic moduli for the oIII and oIV phases. These DFT calculations are carried out using the Projector Augmented Wave (PAW) method [S3] as implemented in the VASP software [S4–S6].

| oIII Wyckoff | $x$ | $y$ | $z$ |
|---|---|---|---|
| Hf(4a) | 0.03361 | 0.26854 | 0.24642 |
| O(4a) | 0.36950 | 0.07420 | 0.11170 |
| O(4a) | 0.73771 | 0.45784 | -0.00211 |

TABLE S4. Wyckoff positions for the oIII phase used in the phonon and elastic properties calculations, with lattice parameters $a$ =5.15999, $b$ =4.95916, $c$ =4.97622, $\alpha$ =90.00000, $\beta$ =90.00000, $\gamma$ =90.00000.

| oIV Wyckoff | $x$ | $y$ | $z$ |
|---|---|---|---|
| Hf(2a) | 0.00000 | 0.76370 | 0.49817 |
| O(2a) | 0.00000 | 0.43314 | 0.16272 |
| O(2a) | 0.00000 | -0.05192 | 0.00453 |

TABLE S5. Wyckoff positions for the oIV phase used in the phonon and elastic properties calculations, with lattice parameters $a$ =3.35777, $b$ =5.05540, $c$ =3.76223, $\alpha$ =90.00000, $\beta$ =90.00000, $\gamma$ =90.00000.

## V. COHERENT EPITAXIAL CONDITION

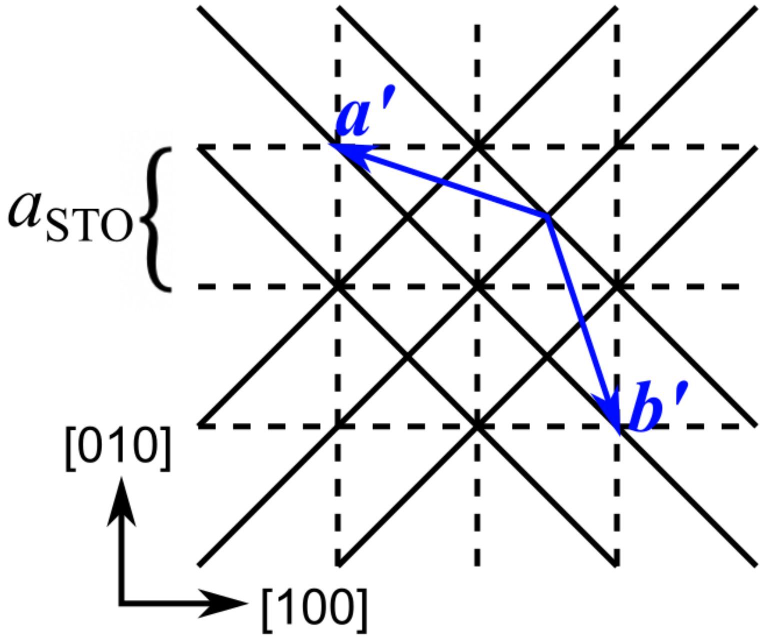


FIG. S2. Orientations of the crystalline axes. The dashed lines correspond to the $[100]_{\mathrm{STO}}$ and $[010]_{\mathrm{STO}}$ directions. The solid lines correspond to the $[110]_{\mathrm{STO}}$ and $[1\text{-}10]_{\mathrm{STO}}$ directions. The blue arrows labeled $\mathbf{a}'$ and $\mathbf{b}'$ correspond to the $a$ and $b$ axes of the (111)–oriented HZO structure.

$\mathbf{a}'$ and $\mathbf{b}'$ are the lattice parameters for the (111)–oriented structure. Here, $(\mathbf{a}', \mathbf{b}', \mathbf{c}') = (\mathbf{a}-\mathbf{c}, \mathbf{c}-\mathbf{b}, \mathbf{a}+\mathbf{b}+\mathbf{c})$ , where $\mathbf{a}$, $\mathbf{b}$, and $\mathbf{c}$ are the lattice parameters for the pseudocubic structure (TABLE S16). In the pseudocubic scheme ($\mathbf{a}//[100]_{\mathrm{HZO}}$, $\mathbf{b}//[010]_{\mathrm{HZO}}$, and $\mathbf{c}//[001]_{\mathrm{HZO}}$), we have $(\mathbf{a}'+\mathbf{b}')//[1\text{-}10]_{\mathrm{HZO}}$ and $(\mathbf{a}'-\mathbf{b}')//[11\text{-}2]_{\mathrm{HZO}}$. In the experiment, the epitaxial condition gives that $[1\text{-}10]_{\mathrm{HZO}}//[1\text{-}10]_{\mathrm{STO}}$, and $[11\text{-}2]_{\mathrm{HZO}}//[110]_{\mathrm{STO}}$. Therefore, we should have $(\mathbf{a}'+\mathbf{b}')//[1\text{-}10]_{\mathrm{STO}}$ and $(\mathbf{a}'-\mathbf{b}')//[110]_{\mathrm{STO}}$ as shown in Fig. S2. Under a coherent epitaxial condition, we have

$$|\mathbf{a}'| = a_{\mathrm{STO}} \times \frac{\sqrt{5}}{\sqrt{2}} = 3.905 \times \frac{\sqrt{5}}{\sqrt{2}} = 6.17\ \text{Å}, \tag{S1}$$

$$\gamma = \arccos\left(\frac{1}{\sqrt{5}}\right) \times 2 = 127^{\circ}. \tag{S2}$$

## VI. SIMULATED XRD

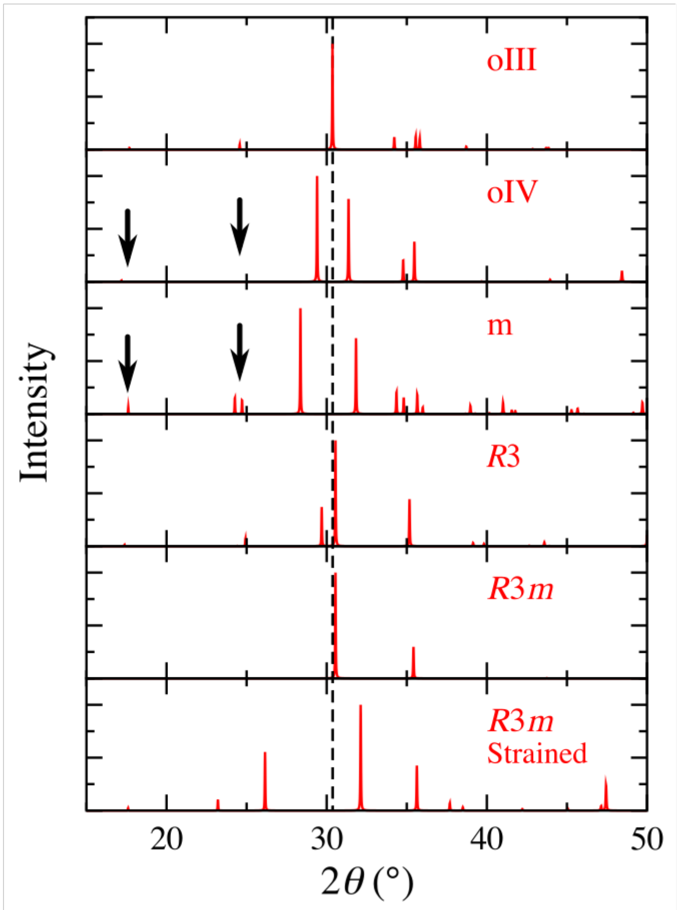


FIG. S3. Simulated x–ray powder diffraction (XRD) for the various competing phases.

FIG. S3 shows the XRD patterns of various ferroelectric phases simulated with the VESTA package [S11]. The dashed line indicates the position of the characteristic peak of the oIII phase. The feature of the ferroelectric phase observed in Ref. [S12] is that its characteristic peak lies to the left of the characteristic peak of the oIII phase. The oIV– and $R3$ phases both satisfy this criterion. However, the energy of the $R3$ phase is high and Zr doping makes it unstable [S12]. The characteristic peak of the $R3m$ phase considered in Ref. [S12] is located at the right of the characteristic peak of oIII phase. The peak of the strained $R3m$ structure, whose polarization matches better with the experimental observation, lies even further right. Here, we would also like to emphasize that even though the XRD pattern of the oIV–phase looks quite like that of the m–phase [S13], there are several features that clearly distinguish the two phases. For example, in oIV there is no peak around 24.5°, and the peak around 17.5° is much weaker than in the m–phase.

FIG. S4 (a) shows the simulated XRD patterns of the competing phases with the thickness $t = 7$ nm. Compared with the bulk patterns, the primary peak of each phase is broadened. There are also oscillations in the intensity due to the finite–size effect. FIG. S5 (b) shows the simulated XRD patterns of the oIV phase, with the thicknesses $t = 7, 9$, and 13 nm. These results match fairly well with the experimental measurements (Figure 1(a) in Ref. [S12]). The small deviations from the experiment indicate that the oIV phase is the predominant phase with a small fraction of other phases.

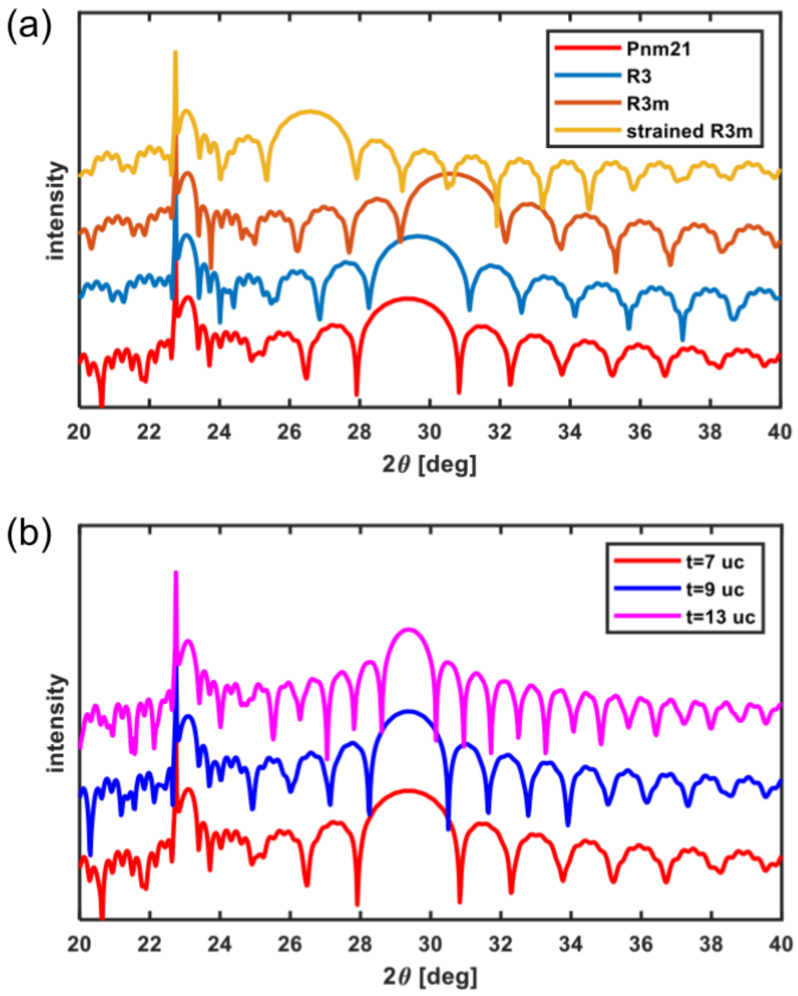


FIG. S4. Simulated x–ray powder diffraction (XRD) for (a) the competing phases with $t = 7$ nm, and (b) the oIV–phase with the 7 nm, 9 nm, and 13 nm thicknesses.

## VII. SIMULATED SAED

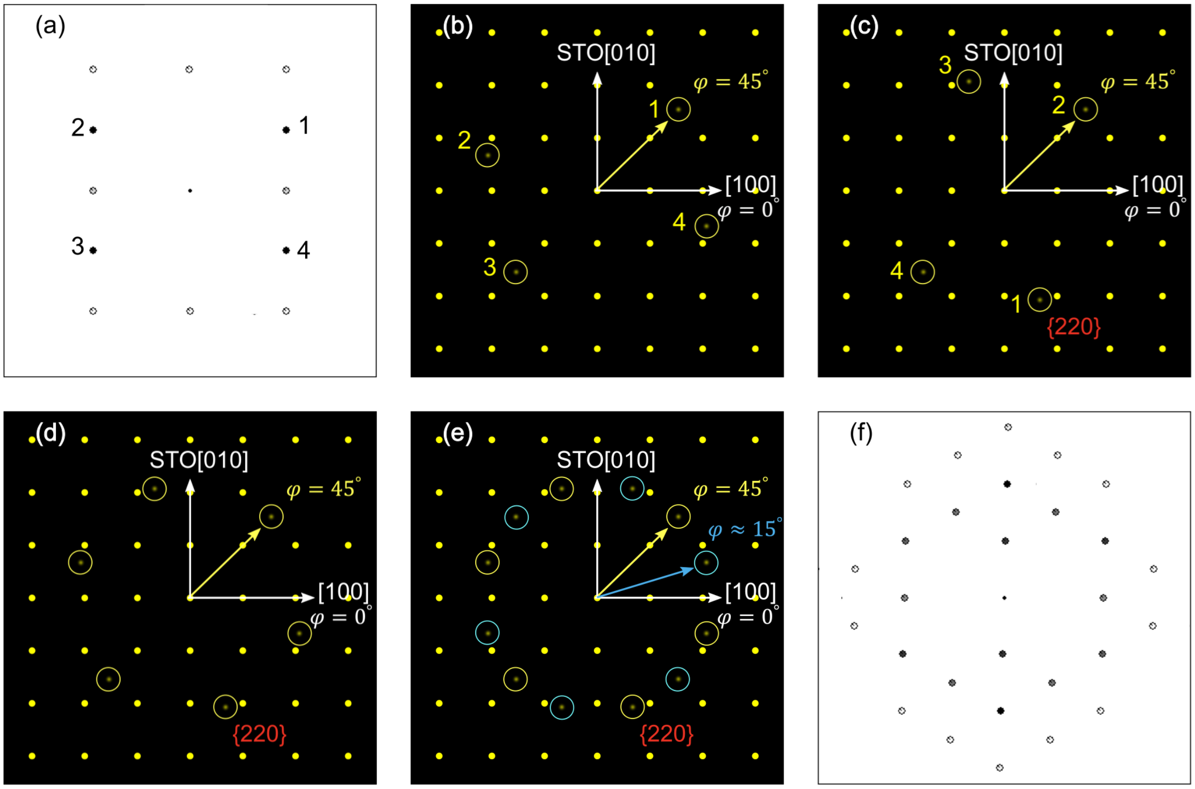


FIG. S5. (a) Simulated Selected–Area Electron Diffraction (SAED) pattern of an 8.4 nm $HfO_2$ thin film in the oIV ($Pnm2_1$) phase. (b) Simulated SAED pattern obtained by matching the spot 1 in (a) to the $\varphi \approx 45^\circ$ one. (c) Simulated SAED pattern obtained by matching the spot 4 in (a) to the $\varphi \approx 45^\circ$ one. In (b) and (c), the square lattice of spots due to the $SrTiO_3$ substrate is also shown. (d) Simulated SAED pattern obtained by merging (b) and (c). (e) Simulated SAED pattern combining all possible domains in the oIV phase. (f) Simulated SAED pattern of a $HfO_2$ thin films in its oIII phase with film thickness $t = 8.4$ nm.

FIG. S5 (a) shows the simulated SAED pattern of single crystalline (111)–oriented $HfO_2$ thin–film in the oIV ($Pnm2_1$) phase. The thickness is 8.4 nm, using the experimental film thickness of 9 nm and taking the thickness of the interfacial t–phase layer to be 0.6 nm. The simulation is carried out with the STEM_CELL package [S14, S15], in which the thickness dependent intensity is estimated by the 2–beam diffraction equation. The structural parameters and atomic coordinates of the oIV–phase in the (111) orientation are listed in TABLE S16. The Debye–Waller factor is taken as 0.01 [S16]. The four spots with the highest intensity correspond to plane distances $d = 1.805$ Å, which is an excellent match with the experimental observation ($d = 1.79$ Å). In the following simulations, we only consider these four spots, assuming that the other low–intensity spots are not visible. In the experimentally observed SAED in Ref. [S12], there is a spot at $\varphi \approx 45^\circ$ due to the lattice orientation given by the epitaxial condition. We can match any of the four brightest spots in FIG. S2 (a) to the $\varphi \approx 45^\circ$ spot, since the four spots are equivalent. Each choice corresponds to a domain with a specific lattice orientation. In FIG. S5 (b) and (c), we match spots 1 and 4 to the $\varphi \approx 45^\circ$ spot respectively, and generate the simulated patterns with the $SrTiO_3$ spots as the background. A total of two different patterns are obtained, since matching spots 1 and 3 (2 and 4) to the $\varphi \approx 45^\circ$ spot gives the same pattern. Then we merge the two patterns into one, as shown in FIG. S5 (e). Next, we note that the substrate has a 4–fold symmetry. Therefore, we can rotate these spots by 90°, and merge the two patterns. The final simulated SAED pattern combining all possible lattice orientations and domains is shown in FIG. S2 (f), This agrees remarkably well with the experimentall observed pattern in Ref. [S12]. For comparison, we also simulated the SAED pattern of an (111)–oriented $HfO_2$ single-crystal thin film in the oIII ($Pca2_1$) phase (structural parameters and atomic coordinates listed in TABLE S19). Though we varied the film thickness in the 6∼9 nm range, we did not get any pattern similar to the experimentally observed one. A typical example with $t = 8.4$ nm is shown in FIG. S5 (f).

## VIII. LATTICE CONSTANTS AND ATOMIC POSITIONS

### A. The Fm$\overline{3}$m cubic (c) structure

| c Wyckoff | $x$ | $y$ | $z$ |
|---|---|---|---|
| Hf(4a) | 0.00000 | 0.00000 | 0.00000 |
| O(8c) | 0.25000 | 0.25000 | 0.25000 |

TABLE S6: Wyckoff positions for the c–phase, with lattice parameters $a$ =5.03694, $b$ =5.03694, $c$ =5.03694, $\alpha$ =90.00000, $\beta$ =90.00000, $\gamma$ =90.00000.

| c pseudocubic | $x$ | $y$ | $z$ |
|---|---|---|---|
| **a** | 5.03694 | 0.00000 | 0.00000 |
| **b** | 0.00000 | 5.03694 | 0.00000 |
| **c** | 0.00000 | 0.00000 | 5.03694 |
| Hf | 0.00000 | 0.00000 | 0.00000 |
| Hf | 0.50000 | 0.00000 | 0.50000 |
| Hf | 0.50000 | 0.50000 | 0.00000 |
| Hf | 0.00000 | 0.50000 | 0.50000 |
| O | 0.75000 | 0.25000 | 0.25000 |
| O | 0.25000 | 0.75000 | 0.25000 |
| O | 0.75000 | 0.75000 | 0.75000 |
| O | 0.75000 | 0.25000 | 0.75000 |
| O | 0.25000 | 0.25000 | 0.25000 |
| O | 0.25000 | 0.75000 | 0.75000 |
| O | 0.25000 | 0.25000 | 0.75000 |
| O | 0.75000 | 0.75000 | 0.25000 |

TABLE S7: Lattice constants and atomic positions of the pseudocubic structure of the c–phase.

| c (111)–oriented | $x$ | $y$ | $z$ |
|---|---|---|---|
| **a** | 7.12327 | 0.00000 | 0.00000 |
| **b** | -3.56163 | 6.16893 | 0.00000 |
| **c** | 0.00000 | 0.00000 | 8.72405 |
| Hf | 0.00000 | 0.50000 | 0.25000 |
| Hf | 0.66667 | 0.83333 | 0.91667 |
| Hf | 0.33333 | 0.16667 | 0.58333 |
| Hf | 0.50000 | 0.00000 | 0.25000 |
| Hf | 0.16667 | 0.33333 | 0.91667 |
| Hf | 0.83333 | 0.66667 | 0.58333 |
| Hf | 0.50000 | 0.50000 | 0.25000 |
| Hf | 0.16667 | 0.83333 | 0.91667 |
| Hf | 0.83333 | 0.16667 | 0.58333 |
| Hf | 0.00000 | 0.00000 | 0.25000 |
| Hf | 0.33333 | 0.66667 | 0.58333 |
| Hf | 0.66667 | 0.33333 | 0.91667 |
| O | 0.16667 | 0.83333 | 0.16666 |
| O | 0.50000 | 0.50000 | 0.50000 |
| O | 0.83333 | 0.16667 | 0.83333 |
| O | 0.33333 | 0.66667 | 0.33333 |
| O | 0.00000 | 0.00000 | 0.00000 |
| O | 0.66667 | 0.33333 | 0.66667 |
| O | 0.83333 | 0.66667 | 0.33333 |
| O | 0.50000 | 0.00000 | 0.00000 |
| O | 0.16667 | 0.33333 | 0.66667 |
| O | 0.66667 | 0.83333 | 0.16666 |
| O | 0.33333 | 0.16667 | 0.83333 |
| O | 0.00000 | 0.50000 | 0.50000 |

| | | | |
|---|---|---|---|
| O | 0.33333 | 0.16667 | 0.33333 |
| O | 0.00000 | 0.50000 | 0.00000 |
| O | 0.66667 | 0.83333 | 0.66667 |
| O | 0.16667 | 0.33333 | 0.16666 |
| O | 0.83333 | 0.66667 | 0.83333 |
| O | 0.50000 | 0.00000 | 0.50000 |
| O | 0.33333 | 0.66667 | 0.83333 |
| O | 0.66667 | 0.33333 | 0.16666 |
| O | 0.00000 | 0.00000 | 0.50000 |
| O | 0.50000 | 0.50000 | 0.00000 |
| O | 0.83333 | 0.16667 | 0.33333 |
| O | 0.16667 | 0.83333 | 0.66667 |

TABLE S8: Lattice constants and atomic positions of the (111)–oriented structure of the c–phase. Here, $(\mathbf{a}', \mathbf{b}', \mathbf{c}') = (\mathbf{a} - \mathbf{c}, -\mathbf{a} + \mathbf{b}, \mathbf{a} + \mathbf{b} + \mathbf{c})$, and the lattice matrix is converted to a lower triangular matrix.

## B. The P4$_2$/nmc tetragonal (t) structure

| t Wyckoff | $x$ | $y$ | $z$ |
|---|---|---|---|
| Hf(2b) | 0.75000 | 0.25000 | 0.75000 |
| O(4d) | 0.25000 | 0.25000 | 0.44293 |

TABLE S9: Wyckoff positions for the t–phase, with lattice parameters $a_0$ =3.56334, $b_0$ =3.56334, $c_0$ =5.19992, $\alpha$ =90.00000, $\beta$ =90.00000, $\gamma$ =90.00000.

| t primitive | $x$ | $y$ | $z$ |
|---|---|---|---|
| $\mathbf{a_0}$ | 3.56334 | 0.00000 | 0.00000 |
| $\mathbf{b_0}$ | 0.00000 | 3.56334 | 0.00000 |
| $\mathbf{c_0}$ | 0.00000 | 0.00000 | 5.19992 |
| Hf | 0.75000 | 0.25000 | 0.75000 |
| Hf | 0.25000 | 0.75000 | 0.25000 |
| O | 0.25000 | 0.25000 | 0.44293 |
| O | 0.75000 | 0.75000 | 0.05707 |
| O | 0.25000 | 0.25000 | 0.94293 |
| O | 0.75000 | 0.75000 | 0.55707 |

TABLE S10: Lattice constants and atomic positions of the primitive cell of the t–phase.

| t pseudocubic | $x$ | $y$ | $z$ |
|---|---|---|---|
| $\mathbf{a}$ | 5.03912 | 0.00000 | 0.00000 |
| $\mathbf{b}$ | 0.00000 | 5.03912 | 0.00000 |
| $\mathbf{c}$ | 0.00000 | 0.00000 | 5.20011 |
| Hf | 0.00000 | 0.00000 | 0.00000 |
| Hf | 0.50000 | 0.00000 | 0.50000 |
| Hf | 0.00000 | 0.50000 | 0.50000 |
| Hf | 0.50000 | 0.50000 | 0.00000 |
| O | 0.25000 | 0.25000 | 0.69295 |
| O | 0.25000 | 0.75000 | 0.30705 |
| O | 0.75000 | 0.75000 | 0.69295 |
| O | 0.75000 | 0.25000 | 0.80705 |
| O | 0.25000 | 0.25000 | 0.19295 |
| O | 0.75000 | 0.75000 | 0.19295 |
| O | 0.75000 | 0.25000 | 0.30705 |
| O | 0.25000 | 0.75000 | 0.80705 |

TABLE S11: Lattice constants and atomic positions of the pseudocubic structure of the t–phase. Here, $(\mathbf{a}, \mathbf{b}, \mathbf{c}) = (\mathbf{a_0} - \mathbf{b_0}, \mathbf{a_0} + \mathbf{b_0}, \mathbf{c_0})$, and the lattice matrix is converted to a lower triangular matrix.

| t (111)–oriented | $x$ | $y$ | $z$ |
|---|---|---|---|
| **a** | 7.23978 | 0.00000 | 0.00000 |
| **b** | -3.73250 | 6.20345 | 0.00000 |
| **c** | -0.22718 | 0.12844 | 8.81859 |
| Hf | 0.00000 | -0.00000 | 0.00000 |
| Hf | -0.00004 | 0.50004 | -0.00008 |
| Hf | 0.49996 | 0.00004 | -0.00008 |
| Hf | 0.50000 | 0.50000 | -0.00000 |
| Hf | 0.33329 | 0.16671 | 0.66658 |
| Hf | 0.33333 | 0.66667 | 0.66667 |
| Hf | 0.83333 | 0.16667 | 0.66667 |
| Hf | 0.83329 | 0.66671 | 0.66658 |
| Hf | 0.16663 | 0.33337 | 0.33325 |
| Hf | 0.16667 | 0.83333 | 0.33333 |
| Hf | 0.66667 | 0.33333 | 0.33333 |
| Hf | 0.66663 | 0.83337 | 0.33325 |
| O | 0.14768 | 0.35233 | 0.10228 |
| O | 0.18565 | 0.81435 | 0.06441 |
| O | 0.68565 | 0.31435 | 0.06441 |
| O | 0.64768 | 0.85233 | 0.10228 |
| O | 0.01895 | 0.98105 | 0.23101 |
| O | 0.98106 | 0.51894 | 0.26904 |
| O | 0.48106 | 0.01894 | 0.26904 |
| O | 0.51895 | 0.48105 | 0.23101 |
| O | 0.01899 | 0.98101 | 0.73108 |
| O | 0.98101 | 0.51899 | 0.76894 |
| O | 0.48101 | 0.01899 | 0.76894 |
| O | 0.51899 | 0.48101 | 0.73108 |
| O | 0.14772 | 0.35228 | 0.60237 |
| O | 0.18562 | 0.81438 | 0.56435 |
| O | 0.68562 | 0.31438 | 0.56435 |
| O | 0.64772 | 0.85228 | 0.60237 |
| O | 0.31434 | 0.18566 | 0.43561 |
| O | 0.35232 | 0.64768 | 0.39775 |
| O | 0.85232 | 0.14768 | 0.39775 |
| O | 0.81434 | 0.68566 | 0.43561 |
| O | 0.31439 | 0.18561 | 0.93571 |
| O | 0.35229 | 0.64772 | 0.89768 |
| O | 0.85229 | 0.14772 | 0.89768 |
| O | 0.81439 | 0.68561 | 0.93571 |

TABLE S12: Lattice constants and atomic positions of the (111)–oriented structure of the t–phase. Here, $(\mathbf{a}', \mathbf{b}', \mathbf{c}') = (\mathbf{a}-\mathbf{c}, \mathbf{c}-\mathbf{b}, \mathbf{a}+\mathbf{b}+\mathbf{c})$, and the lattice matrix is converted to a lower triangular matrix.

### C. The $\mathbf{Pnm2_1}$ orthorhombic (oIV) structure

| oIV Wyckoff | $x$ | $y$ | $z$ |
|---|---|---|---|
| Hf(2a) | 0.00000 | -0.23875 | 0.00206 |
| O(2a) | 0.00000 | 0.43076 | 0.64692 |
| O(2a) | 0.00000 | -0.05685 | 0.50856 |

TABLE S13: Wyckoff positions for the oIV–phase, with lattice parameters $a_0$ =3.42022, $b_0$ =5.15588, $c_0$ =3.75535, $\alpha$ =90.00000, $\beta$ =90.00000, $\gamma$ =90.00000.

| oIV primitive | $x$ | $y$ | $z$ |
|---|---|---|---|
| $\mathbf{a_0}$ | 3.42022 | 0.00000 | 0.00000 |
| $\mathbf{b_0}$ | 0.00000 | 5.15588 | 0.00000 |
| $\mathbf{c_0}$ | 0.00000 | 0.00000 | 3.75535 |

| | | | |
|---|---|---|---|
| Hf | 0.00000 | -0.23875 | 0.00206 |
| Hf | 0.50000 | 0.23875 | 0.50205 |
| O | 0.00000 | 0.43076 | 0.64692 |
| O | 0.50000 | 0.56925 | 0.14692 |
| O | 0.00000 | -0.05685 | 0.50856 |
| O | 0.50000 | 0.05686 | 0.00856 |

TABLE S14: Lattice constants and atomic positions of the primitive cell of the oIV–phase.

| oIV pseudocubic | $x$ | $y$ | $z$ |
|---|---|---|---|
| **a** | 5.07931 | 0.00000 | 0.00000 |
| **b** | 0.47451 | 5.05710 | 0.00000 |
| **c** | 0.00000 | 0.00000 | 5.15555 |
| Hf | 0.00000 | 0.00000 | 0.00000 |
| Hf | 0.50000 | 0.00000 | 0.47744 |
| Hf | 0.00000 | 0.50000 | 0.47744 |
| Hf | 0.50000 | 0.50000 | 0.00000 |
| O | 0.75326 | 0.25324 | 0.29555 |
| O | 0.32249 | 0.32249 | 0.66946 |
| O | 0.25324 | 0.75326 | 0.29555 |
| O | 0.82249 | 0.32248 | 0.80797 |
| O | 0.32248 | 0.82249 | 0.80797 |
| O | 0.75324 | 0.75324 | 0.18190 |
| O | 0.82247 | 0.82247 | 0.66948 |
| O | 0.25325 | 0.25325 | 0.18188 |

TABLE S15: Lattice constants and atomic positions of the pseudocubic structure of the oIV–phase. Here, $(\mathbf{a}, \mathbf{b}, \mathbf{c}) = (\mathbf{c_0} + \mathbf{a_0}, \mathbf{c_0} - \mathbf{a_0}, \mathbf{b_0})$, and the lattice matrix is converted to a lower triangular matrix.

| oIV (111)–oriented | $x$ | $y$ | $z$ |
|---|---|---|---|
| **a** | 7.23757 | 0.00000 | 0.00000 |
| **b** | -4.00517 | 6.02821 | 0.00000 |
| **c** | 0.22359 | -0.11973 | 9.10627 |
| Hf | 0.00000 | 0.00000 | 0.00000 |
| Hf | 0.00750 | 0.49250 | 0.99251 |
| Hf | 0.50750 | -0.00750 | 0.99251 |
| Hf | 0.50000 | 0.50000 | 0.00000 |
| Hf | 0.34084 | 0.15916 | 0.65917 |
| Hf | 0.33334 | 0.66666 | 0.66668 |
| Hf | 0.83334 | 0.16666 | 0.66668 |
| Hf | 0.84084 | 0.65916 | 0.65917 |
| Hf | 0.17417 | 0.32583 | 0.32584 |
| Hf | 0.16667 | 0.83333 | 0.33335 |
| Hf | 0.66667 | 0.33333 | 0.33335 |
| Hf | 0.67417 | 0.82583 | 0.32584 |
| O | 0.15254 | 0.34745 | 0.10072 |
| O | 0.21763 | 0.78237 | 0.10475 |
| O | 0.71763 | 0.28237 | 0.10475 |
| O | 0.65254 | 0.84745 | 0.10072 |
| O | 0.02379 | 0.97620 | 0.22947 |
| O | 0.00479 | 0.49521 | 0.31760 |
| O | 0.50479 | -0.00479 | 0.31760 |
| O | 0.52379 | 0.47620 | 0.22947 |
| O | 0.05097 | 0.94903 | 0.77142 |
| O | 0.98587 | 0.51412 | 0.76738 |
| O | 0.48587 | 0.01412 | 0.76738 |
| O | 0.55097 | 0.44903 | 0.77142 |
| O | 0.17146 | 0.32854 | 0.65094 |
| O | 0.19046 | 0.80953 | 0.56280 |

| | | | |
|---|---|---|---|
| O | 0.69046 | 0.30953 | 0.56280 |
| O | 0.67146 | 0.82854 | 0.65094 |
| O | 0.31921 | 0.18078 | 0.43405 |
| O | 0.38431 | 0.61569 | 0.43809 |
| O | 0.88431 | 0.11569 | 0.43809 |
| O | 0.81921 | 0.68078 | 0.43405 |
| O | 0.33812 | 0.16188 | 0.98426 |
| O | 0.35712 | 0.64287 | 0.89613 |
| O | 0.85712 | 0.14287 | 0.89613 |
| O | 0.83812 | 0.66188 | 0.98426 |

TABLE S16: Lattice constants and atomic positions of the (111)–oriented structure of the oIV–phase. Here, $(\mathbf{a}', \mathbf{b}', \mathbf{c}') = (\mathbf{a} - \mathbf{c}, \mathbf{c} - \mathbf{b}, \mathbf{a} + \mathbf{b} + \mathbf{c})$, and the lattice matrix is converted to a lower triangular matrix.

### D. The Pca2$_1$ orthorhombic (oIII) structure

| oIII Wyckoff | $x$ | $y$ | $z$ |
|---|---|---|---|
| Hf(4a) | 0.466815 | 0.23381 | 0.00000 |
| O(4a) | 0.135205 | 0.43363 | 0.14445 |
| O(4a) | -0.22839 | 0.03651 | 0.25145 |

TABLE S17: Wyckoff positions for the oIII–phase, with lattice parameters $a_0$ =5.23630, $b_0$ =5.01159, $c_0$ =5.04543, $\alpha$ =90.00000, $\beta$ =90.00000, $\gamma$ =90.00000.

| oIII pseudocubic | $x$ | $y$ | $z$ |
|---|---|---|---|
| **a** | 5.04543 | 0.00000 | 0.00000 |
| **b** | 0.00000 | 5.01159 | 0.00000 |
| **c** | 0.00000 | 0.00000 | 5.23630 |
| Hf | 0.00000 | 0.23025 | 0.46605 |
| Hf | 0.50000 | -0.23025 | -0.46605 |
| Hf | 0.00000 | -0.23025 | 0.96605 |
| Hf | 0.50000 | 0.23025 | 0.03395 |
| O | 0.13199 | 0.42406 | 0.12904 |
| O | 0.63199 | -0.42406 | -0.12904 |
| O | 0.13199 | -0.42406 | 0.62904 |
| O | 0.63199 | 0.42406 | 0.37096 |
| O | 0.24856 | 0.04271 | -0.23902 |
| O | 0.74856 | -0.04271 | 0.23902 |
| O | 0.24856 | -0.04271 | 0.26098 |
| O | 0.74856 | 0.04271 | 0.73902 |

TABLE S18: Lattice constants and atomic positions of the primitive and pseudocubic structure of the oIII–phase. Here, $(\mathbf{a}, \mathbf{b}, \mathbf{c}) = (\mathbf{c_0}, \mathbf{b_0}, \mathbf{a_0})$.

| oIII (111)–oriented | $x$ | $y$ | $z$ |
|---|---|---|---|
| **a** | 7.11136 | 0.00000 | 0.00000 |
| **b** | -3.57965 | 6.32934 | 0.00000 |
| **c** | -0.04799 | -0.33706 | 8.82454 |
| Hf | 0.00000 | 0.00000 | 0.00000 |
| Hf | 0.97786 | 0.45573 | 0.02213 |
| Hf | 0.49946 | 0.96653 | 0.03295 |
| Hf | 0.52159 | 0.51079 | 0.01080 |
| Hf | 0.31119 | 0.12239 | 0.68880 |
| Hf | 0.33334 | 0.66668 | 0.66667 |
| Hf | 0.85493 | 0.17747 | 0.67747 |
| Hf | 0.83280 | 0.63320 | 0.69962 |
| Hf | 0.16613 | 0.29987 | 0.36628 |
| Hf | 0.18825 | 0.84413 | 0.34414 |

| | | | |
|---|---|---|---|
| Hf | 0.66666 | 0.33333 | 0.33333 |
| Hf | 0.64453 | 0.78906 | 0.35546 |
| O | 0.19560 | 0.33580 | 0.00418 |
| O | 0.20760 | 0.72699 | 0.12500 |
| O | 0.64874 | 0.31927 | 0.08091 |
| O | 0.68308 | 0.81488 | 0.11965 |
| O | 0.11748 | 0.04674 | 0.21513 |
| O | 0.95239 | 0.34939 | 0.24740 |
| O | 0.53080 | 0.01030 | 0.27195 |
| O | 0.46770 | 0.45718 | 0.26195 |
| O | 0.98207 | 0.98594 | 0.74757 |
| O | 0.01642 | 0.48155 | 0.78631 |
| O | 0.52893 | 0.00247 | 0.67085 |
| O | 0.54093 | 0.39366 | 0.79167 |
| O | 0.19747 | 0.34364 | 0.60528 |
| O | 0.13436 | 0.79052 | 0.59529 |
| O | 0.78414 | 0.38008 | 0.54846 |
| O | 0.61906 | 0.68272 | 0.58073 |
| O | 0.34975 | 0.14821 | 0.45298 |
| O | 0.31541 | 0.65261 | 0.41424 |
| O | 0.87427 | 0.06032 | 0.45834 |
| O | 0.86226 | 0.66913 | 0.33752 |
| O | 0.28573 | 0.01605 | 0.91407 |
| O | 0.45081 | 0.71341 | 0.88180 |
| O | 0.80103 | 0.12385 | 0.92862 |
| O | 0.86413 | 0.67697 | 0.93862 |

TABLE S19: Lattice constants and atomic positions of the (111)–oriented structure of the oIII–phase. Here, $(\mathbf{a}', \mathbf{b}', \mathbf{c}') = (\mathbf{b}-\mathbf{a}, \mathbf{a}-\mathbf{c}, \mathbf{a}+\mathbf{b}+\mathbf{c})$, and the lattice matrix is converted to a lower triangular matrix.

### E. The P$2_1$/c monoclinic (m) structure

| m Wyckoff | $x$ | $y$ | $z$ |
|---|---|---|---|
| Hf(4e) | 0.22468 | -0.04257 | 0.20771 |
| O(4e) | 0.05106 | 0.25698 | -0.02351 |
| O(4e) | 0.43368 | -0.17291 | -0.15081 |

TABLE S20: Wyckoff positions for the m–phase, with lattice parameters $a_0$ = 5.10427, $b_0$ =5.14997, $c_0$ =5.29168, $\alpha$ =90.00000, $\beta$ =80.35428, $\gamma$ =90.00000.

| m (pseudocubic) | $x$ | $y$ | $z$ |
|---|---|---|---|
| **a** | 5.10427 | 0.00000 | 0.00000 |
| **b** | 0.00000 | 5.14997 | 0.00000 |
| **c** | 0.88665 | 0.00000 | 5.21687 |
| Hf | 0.22468 | 0.54257 | 0.70771 |
| Hf | -0.22468 | 0.04257 | -0.20771 |
| Hf | -0.22468 | 0.45743 | 0.29229 |
| Hf | 0.22468 | -0.04257 | 0.20771 |
| O | 0.05106 | 0.24302 | 0.47649 |
| O | -0.05106 | -0.25698 | 0.02351 |
| O | -0.05106 | 0.75698 | 0.52351 |
| O | 0.05106 | 0.25698 | -0.02351 |
| O | 0.43368 | 0.67291 | 0.34919 |
| O | -0.43368 | 0.17291 | 0.15081 |
| O | -0.43368 | 0.32709 | 0.65081 |
| O | 0.43368 | -0.17291 | -0.15081 |

TABLE S21: Lattice constants and atomic positions of the primitive and pseudocubic structure of the m–phase. Here, $(\mathbf{a}, \mathbf{b}, \mathbf{c}) = (\mathbf{a_0}, \mathbf{b_0}, \mathbf{c_0})$.

| m (111)–oriented | $x$ | $y$ | $z$ |
|---|---|---|---|
| **a** | 7.25087 | 0.00000 | 0.00000 |
| **b** | -4.28196 | 6.01581 | 0.00000 |
| **c** | 0.55941 | -0.60024 | 9.43163 |
| Hf | 0.00000 | 0.00000 | 0.00000 |
| Hf | 0.02839 | 0.47161 | 0.97162 |
| Hf | 0.50558 | 0.96050 | 0.04508 |
| Hf | 0.53397 | 0.43212 | 0.01669 |
| Hf | 0.36173 | 0.13827 | 0.63829 |
| Hf | 0.33334 | 0.66666 | 0.66666 |
| Hf | 0.86731 | 0.09878 | 0.68335 |
| Hf | 0.83892 | 0.62717 | 0.71175 |
| Hf | 0.17225 | 0.29384 | 0.37841 |
| Hf | 0.20062 | 0.76545 | 0.35002 |
| Hf | 0.66666 | 0.33333 | 0.33333 |
| Hf | 0.69505 | 0.80495 | 0.30495 |
| O | 0.21539 | 0.35212 | 0.99363 |
| O | 0.20328 | 0.69528 | 0.13836 |
| O | 0.72785 | 0.32976 | 0.09853 |
| O | 0.64410 | 0.76436 | 0.08018 |
| O | 0.99734 | 0.07016 | 0.21167 |
| O | 0.98524 | 0.41333 | 0.35640 |
| O | 0.55653 | 0.00108 | 0.26985 |
| O | 0.47278 | 0.43568 | 0.25150 |
| O | 0.06119 | 0.99643 | 0.76520 |
| O | 0.97743 | 0.43103 | 0.74684 |
| O | 0.54872 | 0.01878 | 0.66029 |
| O | 0.53662 | 0.36195 | 0.80503 |
| O | 0.22321 | 0.33442 | 0.60319 |
| O | 0.13945 | 0.76902 | 0.58483 |
| O | 0.66401 | 0.40349 | 0.54500 |
| O | 0.65192 | 0.74666 | 0.68973 |
| O | 0.31076 | 0.09770 | 0.41351 |
| O | 0.39451 | 0.66310 | 0.43186 |
| O | 0.86995 | 0.02863 | 0.47169 |
| O | 0.88205 | 0.68545 | 0.32696 |
| O | 0.31858 | 0.07999 | 0.02308 |
| O | 0.33068 | 0.73683 | 0.87833 |
| O | 0.80611 | 0.10235 | 0.91816 |
| O | 0.88987 | 0.66775 | 0.93652 |

TABLE S22: Lattice constants and atomic positions of the (111)–oriented structure of the m–phase. Here, $(\mathbf{a}', \mathbf{b}', \mathbf{c}') = (\mathbf{a}-\mathbf{b}, \mathbf{b}-\mathbf{c}, \mathbf{a}+\mathbf{b}+\mathbf{c})$, and the lattice matrix is converted to a lower triangular matrix.


[S1] P. Giannozzi, S. Baroni, N. Bonini, M. Calandra, R. Car, C. Cavazzoni, D. Ceresoli, G. L. Chiarotti, M. Cococcioni, I. Dabo, A. D. Corso, S. de Gironcoli, S. Fabris, G. Fratesi, R. Gebauer, U. Gerstmann, C. Gougoussis, A. Kokalj, M. Lazzeri, L. Martin-Samos, N. Marzari, F. Mauri, R. Mazzarello, S. Paolini, A. Pasquarello, L. Paulatto, C. Sbraccia, S. Scandolo, G. Sclauzero, A. P. Seitsonen, A. Smogunov, P. Umari, and R. M. Wentzcovitch, J. Phys.: Condens. Matter **21**, 395502 (2009).
[S2] H. J. Monkhorst and J. D. Pack, Phys. Rev. B **13**, 5188 (1976).
[S3] P. E. Blöchl, Phys. Rev. B **50**, 17953 (1994).
[S4] G. Kresse and J. Furthmüller, Phys. Rev. B **54**, 11169 (1996).
[S5] G. Kresse and D. Joubert, Phys. Rev. B **59**, 1758 (1999).
[S6] G. Kresse and D. Joubert, Phys. Rev. B **59**, 1758 (1999).
[S7] A. Togo and I. Tanaka, Scr. Mater. **108**, 1 (2015).
[S8] S. Singh, I. Valencia-Jaime, O. Pavlic, and A. H. Romero, Phys. Rev. B **97**, 054108 (2018).
[S9] I. El-Shanshoury, V. Rudenko, and I. Ibrahim, J. Am. Ceram. Soc. **53**, 264 (1970).

[S10] G. I. Csonka, J. P. Perdew, A. Ruzsinszky, P. H. Philipsen, S. Lebègue, J. Paier, O. A. Vydrov, and J. G. Ángyán, Phys. Rev. B **79**, 155107 (2009).
[S11] K. Momma and F. Izumi, J. Appl. Crystallogr. **41**, 653 (2008).
[S12] Y. Wei, P. Nukala, M. Salverda, S. Matzen, H. J. Zhao, J. Momand, A. S. Everhardt, G. Agnus, G. R. Blake, P. Lecoeur, *et al.*, Nat. Mater. **17**, 1095 (2018).
[S13] S. Mueller, C. Adelmann, A. Singh, S. Van Elshocht, U. Schroeder, and T. Mikolajick, ECS J. Solid State Sci. Technol. **1**, N123 (2012).
[S14] V. Grillo and E. Rotunno, Ultramicroscopy **125**, 97 (2013).
[S15] V. Grillo and F. Rossi, Ultramicroscopy **125**, 112 (2013).
[S16] N. Afify, G. Dalba, U. M. K. Koppolu, C. Armellini, Y. Jestin, and F. Rocca, Mater. Sci. Semicond. Process. **9**, 1043 (2006).
